# Supplementary material for: VPTQ: Extreme Low-bit Vector Post-Training Quantization for Large Language Models
Source: arXiv:2409.17066 source file (2024-10-22)
Supplement: Supplementary file 1 [file llama2_2bit_avg_supplement.tex]

\begin{table*}[hbt!]
\setlength{\tabcolsep}{2.5pt}
\centering
\caption{LLaMA-2 2bit quantization results}
\label{tab:llama2_2bit_avg}
\resizebox{1\textwidth}{!}{%
\begin{tabular}{c|ccccccc|ccccccc|ccccccc}
 &
  \multicolumn{7}{c|}{7B} &
  \multicolumn{7}{c|}{13B} &
  \multicolumn{7}{c}{70B} \\
 &
  bit &
  W2↓ &
  C4↓ &
  AvgQA↑ &
  tok/s↑ &
  mem(GB) &
  cost/h↓ &
  bit &
  W2↓ &
  C4↓ &
  AvgQA↑ &
  tok/s↑ &
  mem(GB) &
  cost/h↓ &
  bit &
  W2↓ &
  C4↓ &
  AvgQA↑ &
  tok/s↑ &
  mem/GB &
  cost/h↓ \\ \hline
FP16 &
  16 &
  5.12 &
  6.63 &
  62.2 &
  38.32 &
  27.22 &
  - &
  16 &
  4.57 &
  6.05 &
  65.4 &
  30.03 &
  63.63 &
  - &
  16 &
  3.12 &
  4.97 &
  70.2 &
  multi-gpu &
   &
  - \\
GPTQ &
  2.125 &
  50.75 &
  36.76 &
  39.16 &
  19.59 &
  4.42 &
  0.2 &
  2.125 &
  43.84 &
  23.07 &
  43.72 &
  11.56 &
  7.92 &
  0.3 &
  2.125 &
  NaN &
  NaN &
  59.18 &
  2.38 &
  37.63 &
  2.83 \\
GPTVQ &
  2.25 &
  6.71 &
  9.9 &
  56.14 &
  N/A &
  N/A &
  1.5 &
  2.25 &
  5.72 &
  8.43 &
  61.56 &
  N/A &
  N/A &
  3.7 &
  2.25 &
  4.25 &
  6.9 &
  68.5 &
  N/A &
  N/A &
  12 \\
DB-LLM &
  2.01 &
  7.23 &
  9.62 &
  55.1 &
  N/A &
  N/A &
  N/A &
  2.01 &
  6.19 &
  8.38 &
  59.4 &
  N/A &
  N/A &
  N/A &
  2.01 &
  4.64 &
  6.77 &
  65.8 &
  N/A &
  N/A &
  N/A \\
QuIP\# &
  2 &
  6.19 &
  8.16 &
  58.2 &
  4.4 &
  2.25 &
   &
  2 &
  5.35 &
  7.2 &
  62.0 &
  3.5 &
  3.94 &
   &
  2 &
  3.91 &
  5.71 &
  69.0 &
  1.9 &
  18.36 &
   \\
AQLM &
  2.02 &
  6.64 &
  8.56 &
  56.5 &
  19.4 &
  2.16 &
   &
  1.97 &
  5.65 &
  7.51 &
  60.6 &
  N/A &
   &
   &
  2.07 &
  3.94 &
  5.72 &
  68.8 &
  6.9 &
  18.81 &
  183 \\
AQLM &
  2.29 &
  6.29 &
  8.11 &
  58.6 &
  19.6 &
  2.4 &
  11.07 &
  2.18 &
  5.41 &
  7.2 &
  61.6 &
  16.5 &
  4.14 &
  22.7 &
   &
   &
   &
   &
   &
   &
   \\ \hline
VPTQ &
  2.02 &
  \textbf{6.13} &
  \textbf{8.07} &
  \textbf{58.2} &
  \textbf{39.9} &
  2.28 &
  2 &
  2.02 &
  \textbf{5.32} &
  \textbf{7.15} &
  \textbf{62.4} &
  \textbf{26.9} &
  4.03 &
  3.2 &
  2.07 &
  3.93 &
  5.72 &
  68.6 &
  9.7 &
  19.54 &
  19 \\
VPTQ &
  2.26 &
  \textbf{5.95} &
  \textbf{7.87} &
  \textbf{59.4} &
  \textbf{35.7} &
  2.48 &
  3.1 &
  2.18 &
  \textbf{5.28} &
  \textbf{7.04} &
  \textbf{63.1} &
  \textbf{18.5} &
  4.31 &
  3.6 &
  2.11 &
  3.92 &
  5.71 &
  68.7 &
  9.7 &
  20.01 &
  19
\end{tabular}%
}
\end{table*}
